# Supplementary material for: TipTop: (Almost) Exact Solutions for Influence Maximization in Billion-scale Networks
Source: arXiv:1701.08462 source file (2019-02-07)
Supplement: Supplementary file 1 [file appendix.tex]

\section*{Appendix}
